# Supplementary material for: The effective increase in atomic scale disorder by doping and superconductivity in Ca$_3$Rh$_4$Sn$_{13}$
Source: arXiv:1802.04375 source file (2018-02-12)

# Supplemental information for

## "The effective increase in atomic scale disorder by doping and superconductivity in $\text{Ca}_3\text{Rh}_4\text{Sn}_{13}$ ."

### 1. Variations of lattice parameters refined from Supernova experiments.

(A)  $\text{CaCe}_2\text{Rh}_4\text{Sn}_{13}$

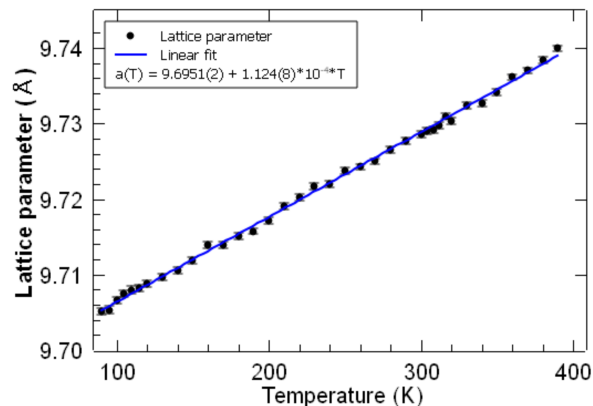

(B)  $\text{Ca}_2\text{Ce}_1\text{Rh}_4\text{Sn}_{13}$

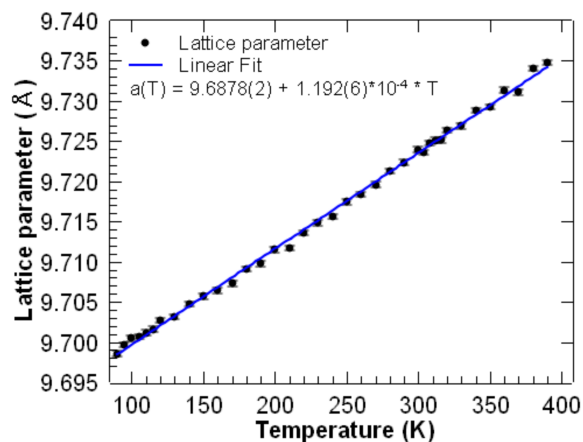

(C)  $\text{CaLa}_2\text{Rh}_4\text{Sn}_{13}$

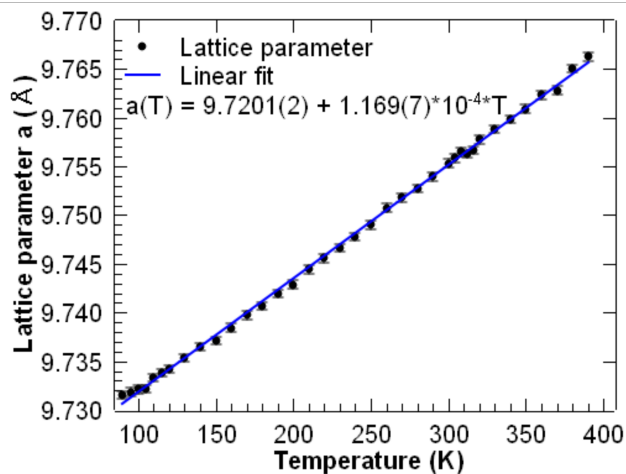

(D)  $\text{Ca}_{2.8}\text{La}_{0.2}\text{Rh}_4\text{Sn}_{13}$

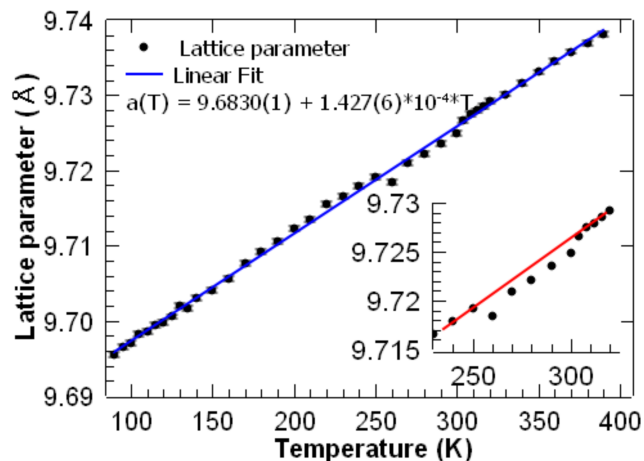

## 2. Variations of Sn2 positional parameters.

CaCe2Rh4Sn13

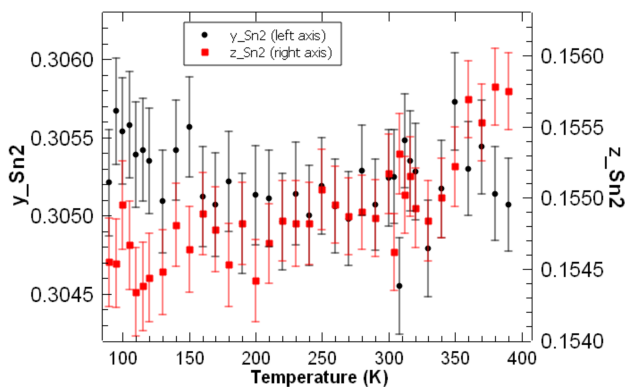

Ca2Ce1Rh4Sn13

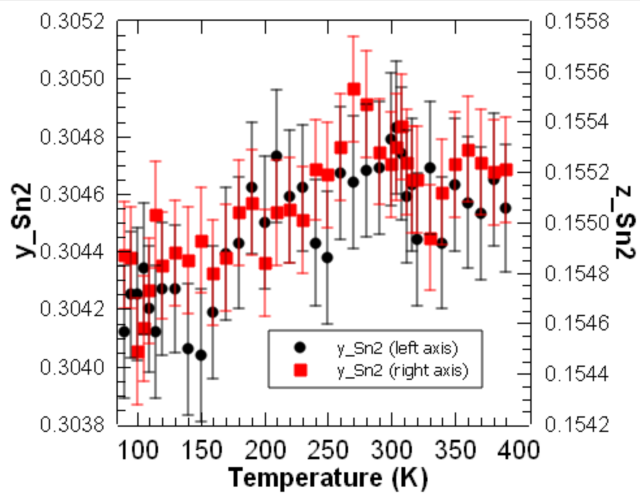

(C) CaLa2Rh4Sn13

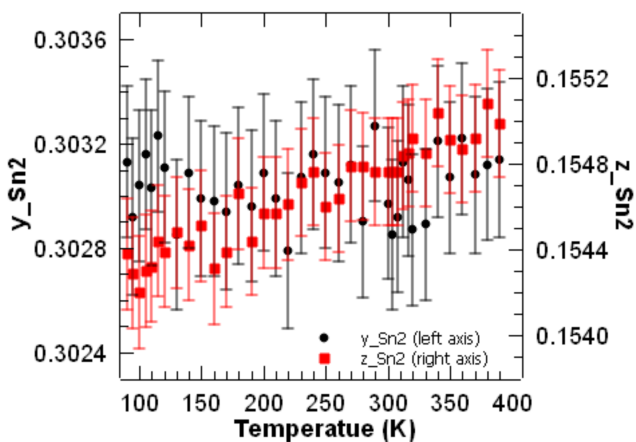

(D) Ca2.8La0.2Rh4Sn13

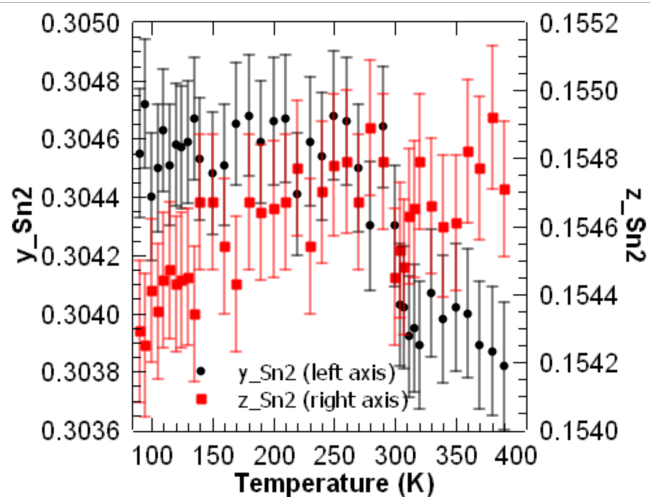

Supplement: Supplementary file 1 [file SI_Plots.pdf]
